# Supplementary material for: Higgs and Goldstone spin-wave modes in striped magnetic texture
Source: arXiv:2110.00882 ancillary file (2021-12-13)
Supplement: Supplementary file 1 [file Supplementary_material_v2.pdf]

# Supplementary Materials for

## Higgs and Goldstone spin-wave modes in striped magnetic texture

Matías Grassi[1], Moritz Geilen[2], Kosseila Ait Oukaci[3], Yves Henry[1], Daniel Lacour[3], Daniel Stoeffler[1], Michel Hehn[3], Philipp Pirro[2], Matthieu Bailleul[1*].

[1]Université de Strasbourg, CNRS, Institut de Physique et Chimie des Matériaux de Strasbourg, UMR 7504, F-67000 Strasbourg, France.

[2] Fachbereich Physik and Landesforschungszentrum OPTIMAS, Technische Universität Kaiserslautern, 67663 Kaiserslautern, Germany.

[3] Institut Jean Lamour, Université de Lorraine, UMR 7198, CNRS, F-54000 Nancy, France.

*Correspondence to: matiasgrassi94@hotmail.com; matthieu.bailleul@ipcms.unistra.fr

## Materials and Methods

Landau theory of stripe nucleation

### Energy functional

The magnetic energy density $E$ for a thin film with perpendicular magnetic anisotropy $K$ subjected to an in-plane external field (geometry shown in Fig. 1(d)) consists of a uniaxial magnetic anisotropy term, an exchange stiffness term, a Zeeman term, and a dipolar term [11]. It reads

$$E = \frac{\mu_0 M_S^2}{2}\left\{-Q n_y^2 + \Lambda^2\left[(\nabla n_x)^2 + \left(\nabla n_y\right)^2 + (\nabla n_z)^2\right] - 2hn_z + \int d\boldsymbol{r}\int d\boldsymbol{r}'\,\boldsymbol{n}(\boldsymbol{r})\overline{\overline{\boldsymbol{G}}}(\boldsymbol{r}-\boldsymbol{r}')\boldsymbol{n}(\boldsymbol{r}')\right\}, \quad \text{(S1)}$$

where $Q = \frac{2K}{\mu_0 M_S^2}$ is the quality factor, $\Lambda = \sqrt{\frac{2A}{\mu_0 M_S^2}}$ is the exchange length, $h = \frac{H}{M_S}$ and $\boldsymbol{n} = \frac{\boldsymbol{M}}{M_S}$ are the normalized external field and normalized magnetization vector, respectively, and $\overline{\overline{\boldsymbol{G}}}(s)$ is the tensorial Green's function of the dipolar interaction.

Considering the stray-field-free-ansatz given in the text, we can rule out the demagnetizing energy (last term of Eq. S1). In addition, we can use the constraint $|\boldsymbol{M}|=M_S$ to rewrite the longitudinal magnetization component ($n_z = \sqrt{1 - n_x^2 - n_y^2}$). Expanding (S1) in powers of $|\psi|$, and averaging over the film thickness and one period of the modulation ($\langle - \rangle = \int_0^\lambda dx \int_{-D/2}^{D/2} dy\, -$), we get [38]

$$\langle E\rangle = \mu_0 M_S^2 h + a(k,h)|\psi|^2 + b(k,h)|\psi|^4 + O(|\psi|^6), \quad \text{(S2)}$$

with

$$a = \frac{\mu_0 M_S^2}{8}\left[-Q\kappa^2 + L^2(\kappa^2+1)^2 + h(\kappa^2+1)\right] \quad \text{(S3)}$$

and

$$b = \frac{\mu_0 M_S^2}{128}\left[L^2(3\kappa^6 + \kappa^4 + \kappa^2 + 3) + \frac{h}{4}(9\kappa^4 + 2\kappa^2 + 9)\right], \quad \text{(S4)}$$

where $\kappa = kD/\pi$ and $L = \Lambda\pi/D$ are two dimensionless ratios governing the stripe texture. Fig. S1(a) shows a plot of the energy density of Eq. S2 for different values of the field.

### Stripe nucleation

Although $b(h,k)$ remains positive for all values considered ($h$>0 here), $a(h,k)$ changes sign for certain values of $k$ and $h$. For a large enough external field $h$, it is clear that $a(h,k)$ is positive whatever the value of $k$ is. The minimum of $<E>$ is therefore obtained for $\psi=0$, which corresponds to the saturated phase. On the contrary, when $h$ decreases below a certain value, there exists a certain range of $k$ for which $a(h,k)$ becomes negative, which correspond to the stripe phase. The nucleation proceeds when the minimum value of $a(h,k)$ as function of $k$ reaches exactly zero. This corresponds to the conditions $a(h_c,k_c) = 0$ and $\frac{\partial a}{\partial k}(h_c,k_c) = 0$, which lead to

$$h_c = Q - 2\sqrt{Q}\frac{\pi}{D}\Lambda, \quad \text{(S5)}$$

$$k_c = \frac{\pi}{D}\sqrt{{Q+h_c}/{Q-h_c}}. \quad \text{(S6)}$$

For the parameters of our films, the corresponding values are $\mu_0 H_c$=10.5 mT and $k_c$=21.6 rad/µm in good agreement with the values obtained by a full micromagnetic simulations of the same system (11.8 mT and 21.9 rad/µm, respectively). This good agreement is expected in the $Q\to 0$ limit [11,39]. The small underestimate results from the approximations made (demagnetizing energy ignored and ansatz not respecting the boundary conditions, see end of next section).

## Stripe evolution

We now proceed by extending the (linear) theory of nucleation to the (non-linear) regime in which the fourth power term plays a role. For this purpose, we assume that the stripe wavenumber does not change as function of the field and keeps the critical value $k_c$. Then, the modulation amplitude $\psi_0$ is deduced by minimizing the average energy density of Eq. S2 (see Fig. S1(a)) as function of $|\psi|$, which leads to

$$\psi_0 = \sqrt{\frac{-a(h,k)}{2b(h,k)}}. \tag{S7}$$

The evolution of modulation amplitude as function of field is shown in Fig. S1(b). This evolution is valid until the point at which the transverse component saturates ($m_y^{\max} = 1$), which corresponds to $\psi_0 = \frac{\pi}{D\,k_c} \cong 0.83$. An extra calculation performed by minimizing numerically the function (S2) with respect to both $|\psi|$ and $k$ shows that the differences do not exceed 10%, which justifies the simplifying assumption made above. Finally, we also compare in Fig. S1(c) the magnetization profiles obtained by mumax3 micromagnetic simulations to those given by the stray-field-free ansatz. One observes a very good agreement, except two deviations: (i) the analytical model somehow underestimates the stripe amplitude (by approximately 10% here), which is not surprising given the approximation made, and (ii) the stray-field-free-ansatz satisfies boundary conditions for the out-of-plane magnetization component of Dirichlet type ($n_y = 0$ at $y = \pm\frac{D}{2}$), whereas the realistic exchange boundary conditions are of Neuman type ($\frac{\partial n_y}{\partial y} = 0$ at $y = \pm\frac{D}{2}$). The simulated $m_y$ profile exhibits an inflection localized in the subsurface region, which allows one to reconcile the two points of view, as explained in [11].

<u>Analytical derivation of spin-wave dispersion close to nucleation</u>

We shall now derive the frequency of spin-waves in the saturated state by extending the stray-field-free ansatz of Eq. 1. The starting point is the Landau-Lifshitz equation describing the precession of the magnetization $\frac{\partial \boldsymbol{M}}{\partial t} = \gamma \boldsymbol{M} \times \frac{\partial E}{\partial \boldsymbol{M}}$, where $E$ is the energy functional of Eq. S1. We linearize it around the saturated equilibrium state $M_s\hat{\boldsymbol{z}}$, and consider a plane-wave of angular frequency $\omega$ and wavenumber $k$ propagating along $\hat{\boldsymbol{x}}$, $\boldsymbol{m}(y)e^{i(\omega t - kx)}$, which leads to an eigenvalue equation [40]

$$i\omega \boldsymbol{m} = \gamma \mu_0 M_s \hat{\boldsymbol{z}} \times \left\{ h\boldsymbol{m} + \Lambda^2\left(k^2 + \frac{\partial^2}{\partial y^2}\right)\boldsymbol{m} + Q m_z \hat{\boldsymbol{z}} + \int_{-D/2}^{D/2} dy' \overline{\overline{\boldsymbol{G}}}_k(y-y')\boldsymbol{m}(y') \right\}. \tag{S8}$$

Here $\overline{\overline{\boldsymbol{G}}}_k$ is a 2×2 tensor acting in the *(x,y)* plane, as obtained by a Fourier transform of $\overline{\overline{\boldsymbol{G}}}(s)$. Eq. S8 is an integro-differential equation which cannot be solved analytically unless some approximations are made. To proceed, we shall follow the Kalinikos-Slavin method, which consists in projecting this equation over a suitable basis set and solving the resulting matrix equation in a perturbation approach [27]. Usually, this basis set consists of the series of exchange-dominated standing wave modes which are the solutions of the scalar differential equation obtained when neglecting the last term of Eq. S8. In the absence of any surface contribution to the magnetic energy functional for the corresponding component, these standing waves are unpinned (Neuman boundary conditions). On the contrary, in the presence of a strong surface anisotropy disfavoring this component, the standing waves are pinned (Dirichlet boundary conditions). In the following, we shall adapt this treatment by using a different basis set derived in the opposite limit in which the dipole interaction plays a leading role rather than the exchange one. This basis set is sketched

in Fig. 2(a), it consists of the two vector functions that form the static ansatz of Eq. 1, namely $\boldsymbol{S}_x(y) = \sin\left(\frac{\pi}{D}y\right)\hat{\boldsymbol{x}}$ and $\boldsymbol{C}_y(y) = \cos\left(\frac{\pi}{D}y\right)\hat{\boldsymbol{y}}$ (thin blue and red bars, respectively), complemented by two functions obtained by a 90° rotation of them, namely $\boldsymbol{S}_y(y) = \sin\left(\frac{\pi}{D}y\right)\hat{\boldsymbol{y}}$ and $\boldsymbol{C}_x(y) = \cos\left(\frac{\pi}{D}y\right)\hat{\boldsymbol{x}}$ (thick blue and red bars, respectively). In the Kalinikos-Slavin language, $\boldsymbol{S}_x$ and $\boldsymbol{S}_y$ are unpinned while $\boldsymbol{C}_x$ and $\boldsymbol{C}_y$ are pinned. Such combination, which would not make sense in the exchange-dominated limit, is justified by the leading role of the dipolar interaction in our case, which promotes a certain combination of $\boldsymbol{S}_x$ and $\boldsymbol{C}_y$, so as to achieve flux closure, while small components along $\boldsymbol{S}_y$ and $\boldsymbol{C}_x$ naturally arise from the precession of the magnetization.

Let us write the complex amplitude precession $\boldsymbol{m} = s\boldsymbol{S}_x + s'\boldsymbol{S}_y + c'\boldsymbol{C}_x + c\boldsymbol{C}_y$ and project the Landau-Lifshitz equation Eq. (S8) over each basis vector. This results in a matrix equation:

$$\begin{pmatrix} -i\Omega & \Omega_{sy} & -i2Q_{sc} & 0 \\ -\Omega_{sx} & -i\Omega & 0 & i2Q_{sc} \\ -i2Q_{sc} & 0 & -i\Omega & \Omega_{cy} \\ 0 & i2Q_{sc} & -\Omega_{cx} & -i\Omega \end{pmatrix}\begin{pmatrix} s \\ s' \\ c' \\ c \end{pmatrix} = 0, \tag{S9}$$

where $\Omega = \frac{\omega}{\gamma\mu_0 M_S}$ is the normalized frequency, while $\Omega_{(s,c)x} = h + \Lambda^2\left(k^2 + \frac{\pi^2}{D^2}\right) + P_{(s,c)}$ and $\Omega_{(s,c)y} = h + \Lambda^2\left(k^2 + \frac{\pi^2}{D^2}\right) + 1 - P_{(s,c)} - Q$ are normalized Kittel pseudo-frequencies corresponding to each of the basis functions. Here $P_s = \frac{k^2D^2}{\pi^2+k^2D^2}\left[1 - \frac{2k^2D^2}{\pi^2+k^2D^2}\frac{1+e^{-|k|D}}{|k|D}\right]$ and $P_c = \frac{k^2D^2}{\pi^2+k^2D^2}\left[1 + \frac{2\pi^2}{\pi^2+k^2D^2}\frac{1+e^{-|k|D}}{|k|D}\right]$ are self-demagnetizing factors relative to $\boldsymbol{S}_x$ and $\boldsymbol{C}_x$ , respectively, while $Q_{sc} = \frac{\pi kD}{2(\pi^2+k^2D^2)^2}\{\pi^2 + |k|D[|k|D - 2(1+e^{-|k|D})]\}$ is a mutual demagnetizing factor describing the coupling between $\boldsymbol{S}_x$ and $\boldsymbol{C}_y$ (or $\boldsymbol{S}_y$ and $\boldsymbol{C}_x$) [38].

The eigenfrequencies of Eq. S9 are found by nulling the determinant of the matrix [41], which provides us with two values

$$\Omega_{0,1}^2 = \frac{\Omega_{sx}\Omega_{sy} + \Omega_{cx}\Omega_{cy}}{2} - Q_{sc}^2 \mp \frac{1}{2}\sqrt{\left(\Omega_{sx}\Omega_{sy} - \Omega_{cx}\Omega_{cy}\right)^2 + 4Q_{sc}^2(1 - 2P_s - Q)(1 - 2P_c - Q)}. \tag{S10}$$

The dispersion relations corresponding to these two roots are shown in Fig. S2(a) as thick solid lines, together with all the spin-wave modes calculated by solving numerically a finite-difference version of Eq. S8 [42] (thin lines). One recognizes clearly that the low frequency root corresponds to the soft mode. The second root reproduces quite well the mode with a high positive group velocity, which we identify to a conventional Damon-Eshbach spin-wave branch [26] whose frequency is dominated by the strong dipole fields it generates. Fig. S2(b) shows the field dependence of the eigenvectors at the critical wave-vector $k_c$. One clearly distinguishes a vanishing of the small components *s'* and *c'* at the critical field. Besides, the ratio *s*/*c* is of a magnitude close to the value $\frac{\pi}{Dk_c} \cong 0.83$, and is purely imaginary (not shown). These features correspond to the picture of a magnetic flux-closed nucleation mode as described by Eq. 1.

<u>Determination of the frequency of the Higgs mode</u>

Near the nucleation point, the lowest frequency mode is therefore dominated by a specific combination of components $\boldsymbol{S}_x$ and $\boldsymbol{C}_y$. We can group the dynamic magnetization components into this combination and the complementary one containing $\boldsymbol{S}_y$ and $\boldsymbol{C}_x$:

$$m_\psi(y) = s\boldsymbol{S}_x(y) + c\boldsymbol{C}_y(y), \qquad \text{(S11)}$$
$$m_\tau\,(y) = s'\boldsymbol{S}_y(y) + c'\boldsymbol{C}_x(y).$$

The coordinate $m_\psi$ approximates the ansatz and $m_\tau$ is perpendicular to it. Because $m_\psi$ corresponds to a nearly stray-field free distribution, the effective field it generates is dominated by the anisotropy, exchange and Zeeman contributions (see Eq. S8). All these contributions have the same spatial profiles and direction as the basis vectors, which allows one to write the corresponding effective field as $\frac{\partial^2 E}{\partial {m_\psi}^2} m_\psi$ (no $m_\tau$ component). This allows one to write the precession frequency as a Kittel formula with no crossed terms [43], as in the case of the uniform (*k=0*) precession in a thin film. It reads

$$f = \frac{\gamma M_S}{2\pi}\sqrt{\frac{\partial^2 E}{\partial {m_\psi}^2}\frac{\partial^2 E}{\partial {m_\tau}^2}}\ . \qquad \text{(S12)}$$

The description in the frame defined by $\psi$ and $\tau$ is quite useful, as we know that the critical behavior is restricted to $m_\psi$. The energy variation as a function of $m_\psi$ can be approximated by expression S2, which can be used to calculate $\frac{\partial^2 E}{\partial {m_\psi}^2}$, as the variable $\psi$ approximates the component $m_\psi$. If $H$>$H_c$, the minimum is located at $|\psi| = 0$ and the curvature is given by $2a(k_c, h)$. On the other hand, if $H$<$H_c$, the point at $|\psi| = 0$ becomes a maximum with curvature $-2a(k_c, h)$ and the minimum is located at $|\psi| = \psi_0$ (see S7). The second derivative at this point can be calculated from Eq. S2 as $\frac{\partial^2 E}{\partial {m_\psi}^2}|_{\psi_0} = 4a(k_c, h)$. On the other hand, the transversal curvature $\frac{\partial^2 E}{\partial {m_\tau}^2}$ is dominated by the dipolar field created by the magnetic charges and does not depend significantly on the value of $|\psi|$.

The Kalinikos-Slavin method, by construction, determines the frequency associated with the perturbations of the uniform state, or what is the same, $|\psi| = 0$. Below the critical field, the frequency calculated at the critical wavevector becomes imaginary (Fig. 2(b)), which indicates that one of the curvatures in Eq. S12 is negative, as schematically shown in Fig. S3. Although this precession around an unstable point is not physical, its frequency can be used to calculate the real frequency of the mode at the minimum. Using expression S12 and the relations between $\frac{\partial^2 E}{\partial {m_\psi}^2}$ at the saddle point and at the minumum, the Higgs frequency is $\omega|_{\psi_0} = -i\sqrt{2}\omega|_0$, where $\omega|_0$ is the frequency calculated with the Kalinikos-Slavin method explained in the previous section.

<u>Film fabrication, structural and magnetic characterization</u>

We deposited Ta5nm/$Co_{40}Fe_{40}B_{20}$180nm/Pt5nm films onto intrinic silicon substrate by magnetron sputtering. The films are amorphous as deduced from X-ray scattering and transmission electron microscopy. Vibrating sample magnetometry allows one to determine the hysteresis cycle (Fig. 1(b)) and the saturation magnetization ($M_s$=1330±30 kA/m). We conducted ferromagnetic resonance measurements over a broad range and frequency (1-50 GHz) and field (0-2.7 T), applied

both in the film plane and perpendicular to it. This allowed us to extract the gyromagnetic ratio ($\gamma/2\pi$=29.9±0.2 GHz/T), the damping constant ($\alpha$=0.005) and the exchange stiffness constant ($A$=16.6±0.1 pJ/m), which was extracted from the position of a set of five perpendicular standing spin wave resonances [38,44]. Magnetic force microscopy images were recorded as function of the in-plane field, confirming the appearance of a well-ordered stripe texture below a field of about 12 mT. From the wavelength of the stripe texture and from the value of the nucleation field, we estimate a value of the perpendicular magnetic anisotropy of $K$=32.7±2 kJ/m$^3$, in good agreeement with the value deduced from ferromagnetic resonance. This uniaxial anisotropy is associated to magnetolastic effects [45], as often encountered in amorphous ferromagnetic films [46].

Brillouin light scattering measurements

We performed Brillouin light scattering (BLS) measurements in the conventional thermal-excitation mode at room temperature. The film was placed in the gap of an electromagnet, and a p-polarized laser beam of a power of about 200 mW was focused on its surface over a spot of about 40 µm. Measurements were performed in the Voigt configuration with a varying angle of incidence $\theta_i$. The s-polarized component of the backscattered light was frequency-analyzed used a Tandem-Fabry-Pérot interferometer.

A typical spectrum for the saturated state is shown in Fig. S4(a), which displays the scattering intensity as function of transferred frequency for a field of 30 mT, a laser wavelength of 532 nm and an angle of incidence of 21° (k=8.5 rad/µm). One recognizes five peaks located symmetrically at negative and positive transferred frequencies (Stokes and anti-Stokes). To recover the spin-wave dispersion, the angle of incidence was varied using a motorized stage. Fig. S4(b) shows a color plot of the recorded scattering intensity as function of transferred wavenumber and frequency. One recognizes five branches. The lowest frequency one is identified to the soft mode precursor of stripe nucleation, while the four higher frequency ones are to be identified to perpendicular standing spin-wave modes of increasing order [47]. Lines in Fig. 3(b) are obtained using a finite difference diagonalization code [42]. Fig. 2(c) shows the same data, although on a smaller frequency range, and with the Stokes and anti-Stokes sides combined together to simplify visualization.

A typical spectrum for the stripe phase is shown in Fig. S5(a), which displays the scattering intensity as function of transferred frequency for a field of 7 mT, a laser wavelength of 532 nm and an angle of incidence of 22° (k=9 rad/µm). There, although the signal is weaker than in the saturated state, one recognizes two peaks: a low frequency peak at about 3.5GHz, visible both on the Stokes and anti-Stokes side, and a high frequency peak at about 5 GHz, visible on the anti-Stokes side. These two modes can be followed as function of the transferred wave-vector, as shown in the color plot of Fig. S5(b), allowing one to extract the peak positions shown in Fig. 3(a) as circles and squares.

In order to increase the sensitivity at high wavevectors, the measurements shown in Fig. 3 (g) were performed at a laser wavelength of 451 nm. To obtain these data, the angle incidence was fixed at 50º (21.1 rad/ µm) while decreasing the magnetic field from 30 mT.

FMR measurements

We performed broadband ferromagnetic resonance measurements by placing a portion of film on top of a microwave transmission line and measuring the change of its transmission coefficient as function of field and frequency. The coupling geometry is shown in Fig. S6(a): The transmission line consists of a channelized coplanar waveguide (cCPW) board with a center conductor of a width $W$=300 µm. A 2 mm long portion of ferromagnetic film is placed against it. The film surface is in contact with the ground plane of the cCPW, which lies $R$=20 µm above the center track, to avoid short circuit. The cCPW is connected to a vector network analyzer using coplanar launchs and coaxial cables. A Through Reflect Line on-board calibration is performed prior to measurements. We determine the effective permeability $\mu_{eff}$ of the portion of waveguide loaded by the ferromagnetic film by applying the Nicholson-Ross-Weir algorithm to the de-embedded microwave $S$ parameters [48]. The effective susceptibility $\chi_{eff}$ is obtained by substracting a reference measurement taken at a high field $H_{ref}$ : $\chi_{eff}(H)= \mu_{eff}(H)-\mu_{eff}(H_{ref})$.

Figure S6(b) shows the imaginary part of the effective susceptibility measured in the conventional transverse pumping configuration (H oriented in the film plane, parallel to the cCPW axis). One recognizes a clear absorption line, attributed to the uniform precession mode of the film (i.e. the k~0 lowest frequency in Fig. S2(a)). Figure S6(c) shows the imaginary part of the effective susceptibility measured in the longitudinal pumping configuration ($H$ oriented in the film plane, perpendicular to the cCPW axis), of direct interest for the measurement of the Higgs mode (same data as in Fig. 3(f), but over a larger field and frequency range). In addition to the Higgs mode (whose frequency decreases to very small values on approaching the critical field), one recognizes an additional absorption line whose frequency increases as function of field intensity [38]. This lies at the same position as the main FMR line of Fig. S6(b), which allows one to interpret it as a conventional FMR absorption related to a small fraction of the pumping field that is not parallel to H (vertical inflection of the field lines of $\boldsymbol{h}_1$ in Fig. S6(a)).

Micromagnetic simulations

We conducted finite-difference micromagnetic simulations using mumax3 [30]. The unit cell of the stripe texture is divided into 100x60x1 cells of size 2.87x3x5 nm$^3$. The computing volume contains 115 such unit cells into the $x$ direction. To emulate an extended film, we use periodic boundary conditions with (1,0,110000) repeats, such that the total volume taken into account for determining the dipolar field is 100x0.18x1100 µm$^3$. The equilibrium stripe texture is obtained by reducing progressively the applied field H from the saturated state, as an equilibrium solution of the Landau-Lifshitz-Gilbert equation, first with a Gilbert damping value $\alpha$=0.5, then for values reduced progressively to 0.005.

The spin-wave dispersion relations are obtained by a spatial ($x$ axis) and time Fourier transform of the surface vertical dynamic magnetization $m_y(y=+D/2)$ recorded during 50 ns after application of a localized $y$-oriented magnetic field pulse (amplitude=50 mT, duration=20 ps, extension=the two central columns of cells along the $x$ direction).

From these calculations, we also obtain the dynamic tranverse components of the different modes, as shown in Figs. 3(d,e). We can also determine the dynamic longitudinal components of the modes. An example of these profiles for $\mu_0$H=7 mT is shown in Fig. S7. It is possible to recognize that the Higgs mode has a non-vanishing integral in one stripe period. This implies that it is visible in a longitudinal pumping FMR experiment, which explains the observation of Fig. 3(f). In

contrast, the longitudinal component of the Goldstone mode presents a vanishing integral over one period, thus it is invisible to FMR.

## References

[38] M. Grassi, "*Spin waves in inhomogeneous magnetization distributions*", thesis, Université de Strasbourg (2021)

[39] G. Asti, M. Ghidini, M. Mulazzi, R. Pellicelli, M. Solzi, K. Chesnel, A. Marty, Nucleation of weak stripe domains: Determination of exchange and anisotropy thermal variation. *Phys. Rev. B* **76**, 094414 (2007)

[40] A.G. Gurevich, G.A. Melkov, *Magnetization Oscillations and Waves* (CRC Press, 1996)

[41] M. Grassi, M. Geilen, D. Louis, M. Mohseni, T. Brächer, M. Hehn, D. Stoeffler, M. Bailleul, P. Pirro, Y. Henry, Slow-Wave-Based Nanomagnonic Diode. *Phys. Rev. Applied* **14**, 024047 (2020)

[42] Y. Henry, O. Gladii, M. Bailleul, Propagating spin-wave normal modes: A dynamic matrix approach using plane-wave demagnetizating tensors. arXiv:1611.06153 (2016)

[43] H. Y. Yuan, R. A. Duine, Universal field dependence of magnetic resonance near zero frequency. *Phys. Rev. B* **103**, 134440 (2021).

[44] P. Talagala, P.S. Fodor, D. Haddad, R. Naik, R., L. E. Wenger, P.P. Vaishnava, V. M. Naik, Determination of magnetic exchange stiffness and surface anisotropy constants in epitaxial $Ni_{1-x}Co_x$ (001) films. *Phys. Rev. B* **66**, 144426 (2002)

[45] K. Ait Oukaci, "*Periodic magnetic domain structures for channeled spin waves propagation*", thesis, Université de Lorraine, Nancy (2021)

[46] G. Suran, M. Naili, H. Niedoba, F. Machizaud, O. Acher, D. Pain, Magnetic and structural properties of Co-rich CoFeZr amorphous thin films. J. Magn. Magn. Mater. 192, 443-457 (1999)

[47] Grünberg, P., Mayr, C., Vach, W., Grimsditch, M. Determination of magnetic parameters by means of Brillouin Scattering. Examples: Fe, Ni, Ni0.8Fe0.2. Journal of Magnetism and Magnetic Materials, 28, 319–325 (1982).

[48] C. Bilzer, T. Devolder, P. Crozat, C. Chappert, Vector network analyzer ferromagnetic resonance of thin films on coplanar waveguides: Comparison of different evaluation methods. *J. Appl. Phys.* **101**, 074505 (2007)

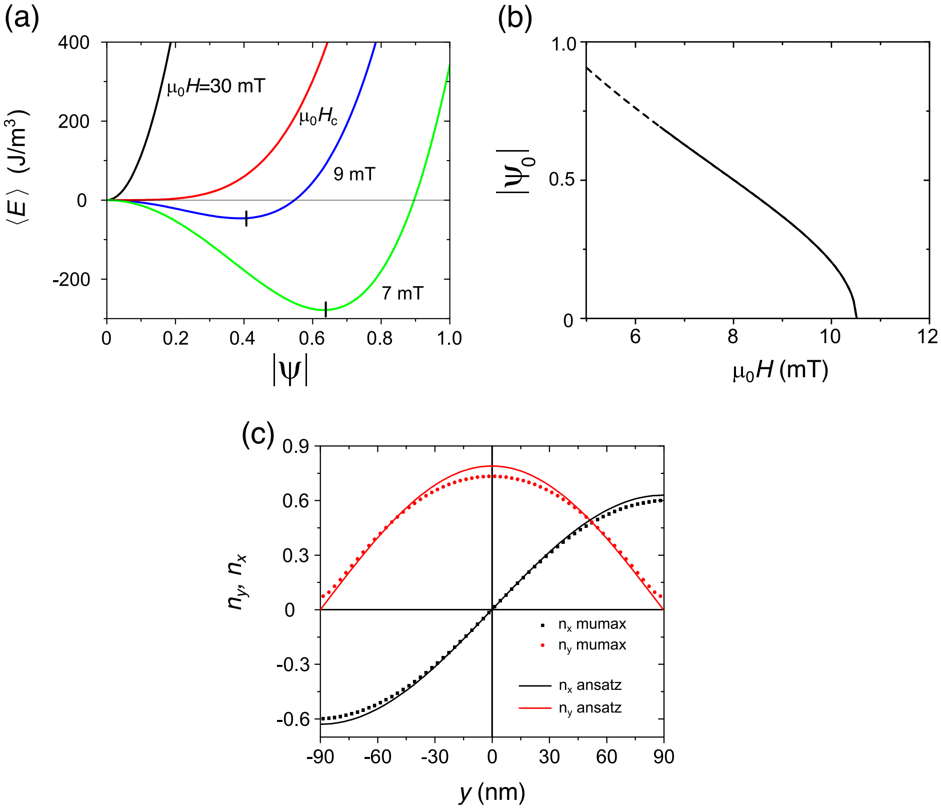


Fig. S1. Landau theory of weak stripes texture. (a) Evolution of the energy functional as function of the applied field. (b) Equilibrium value of the module of the order parameter extracted from the minimization of the energy functionals as shown in panel (a). The range where this approach is valid (when $|\boldsymbol{M_y}| < \boldsymbol{M_S}$) is indicated by the solid line. (c) Comparison of the stripe ansatz (Eqs. 1 and S5-7) with the magnetization profile obtained by mumax3 micromagnetic simulations, both at $\mu_0 H = 7$ mT**.**

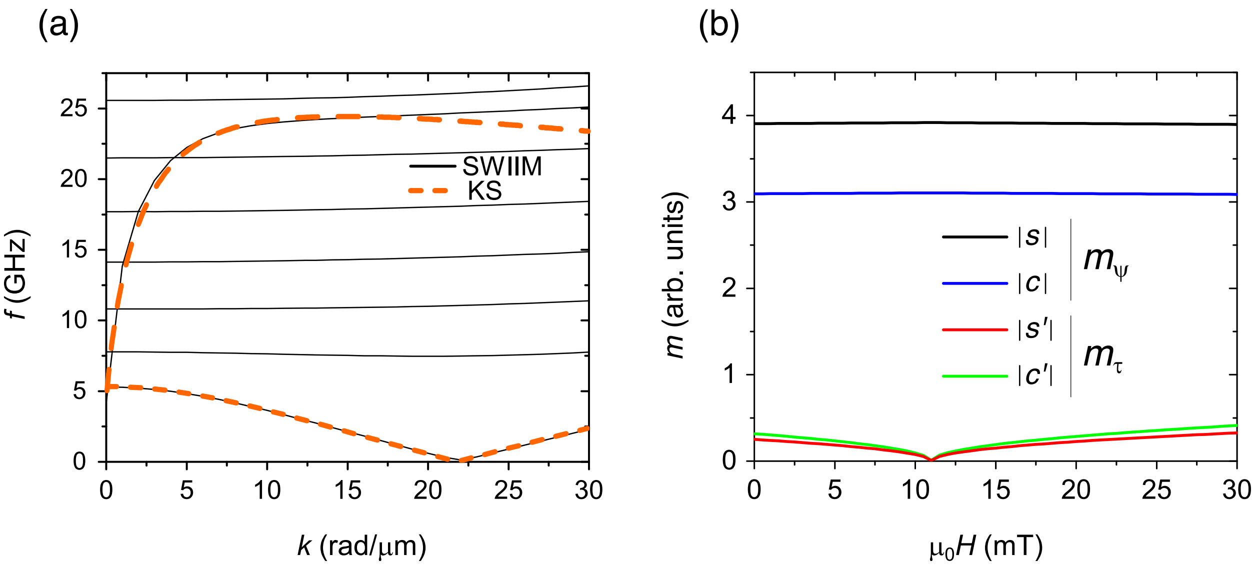


Fig. S2. Normal mode analysis in the saturated state. **(a)** Eigenfrequencies determined at the critical field using the Kalinikos-Slavin method (KS, Eq. S10) and a finite difference simulation [SWIIM, [42]]. (b) Modulus of the four components of the eigenvector of Eq. S9 corresponding to the lowest frequency mode at $k$=21.1 rad/ μm as function of the applied field.

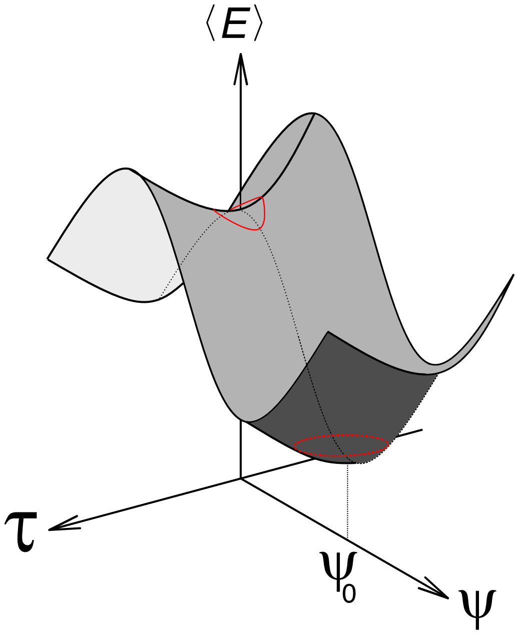


Fig. S3. Sketch of the energy surface as function of the two orthogonal magnetization coordinates τ and ψ (Eq. S11) for an applied field lower than the critical field. We observe that the uniform state ($\tau = \psi = 0$) defines an unstable saddle point, while the minimum is located at $\psi = \psi$ and $\tau = 0$.

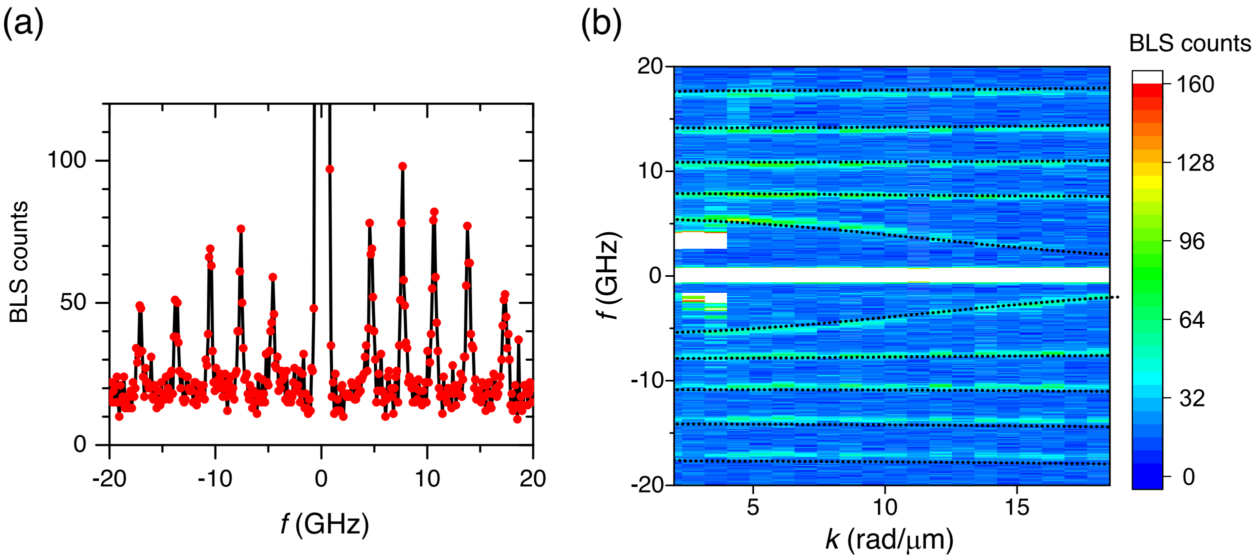


Fig. S4. Measured Brillouin light scattering signals in the saturated state ($\mu_0 H$=14 mT). (a) Plot of the inelastic light scattering intensity as function of transferred frequency for an angle of incidence of 21° (8.5 rad/μm). (b) Color plot of the BLS signal as function of transferred wave-vector and transferred frequency. The dotted lines are the dispersions of the five lowest frequency spin-wave modes deduced from a finite difference calculation [42].

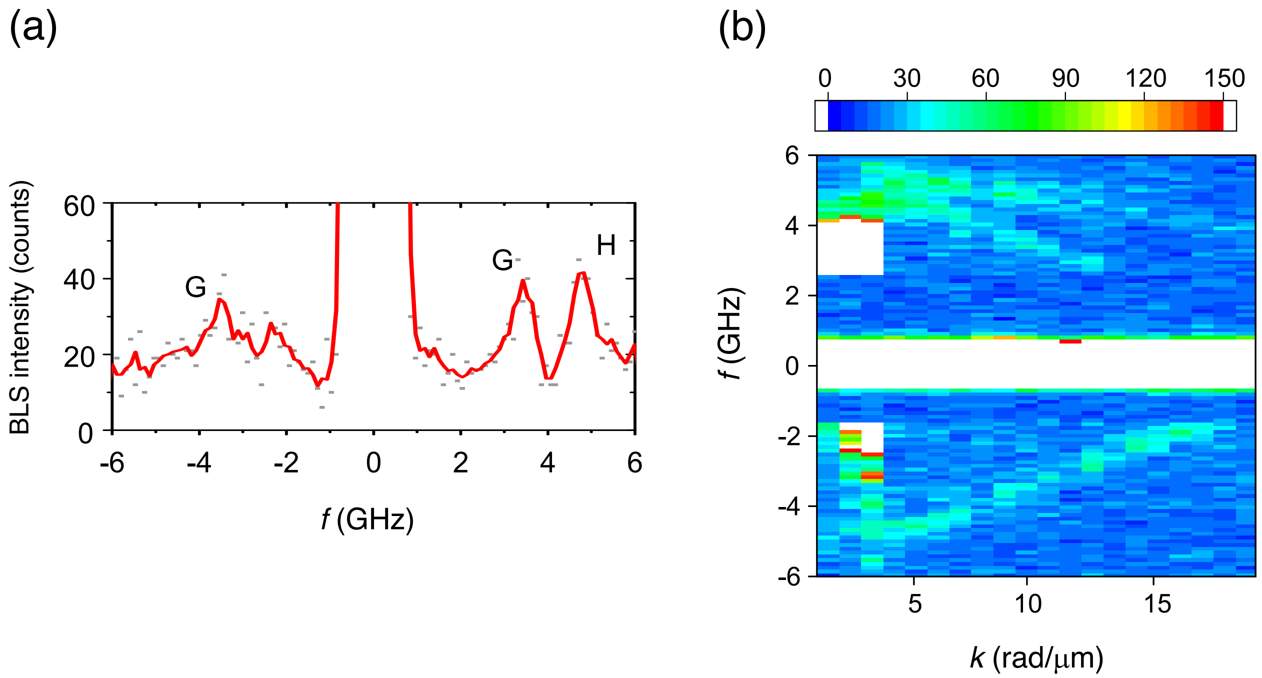


Fig. S5. Measured Brillouin light scattering signals in the stripe phase ($\mu_0 H$=7 mT). (a) Plot of the BLS intensity as function of transferred frequency for an angle of incidence of 22° (9 rad/µm). Letters G and H refers to the Goldstone and the Higgs branches, respectively. The raw data points are shown in gray, while the red line shows a three-point average. (b) Color plot of the BLS signal as function of transferred wave-vector and transferred frequency. The positions of the corresponding peaks are reported in Fig. 3a as circles and squares.

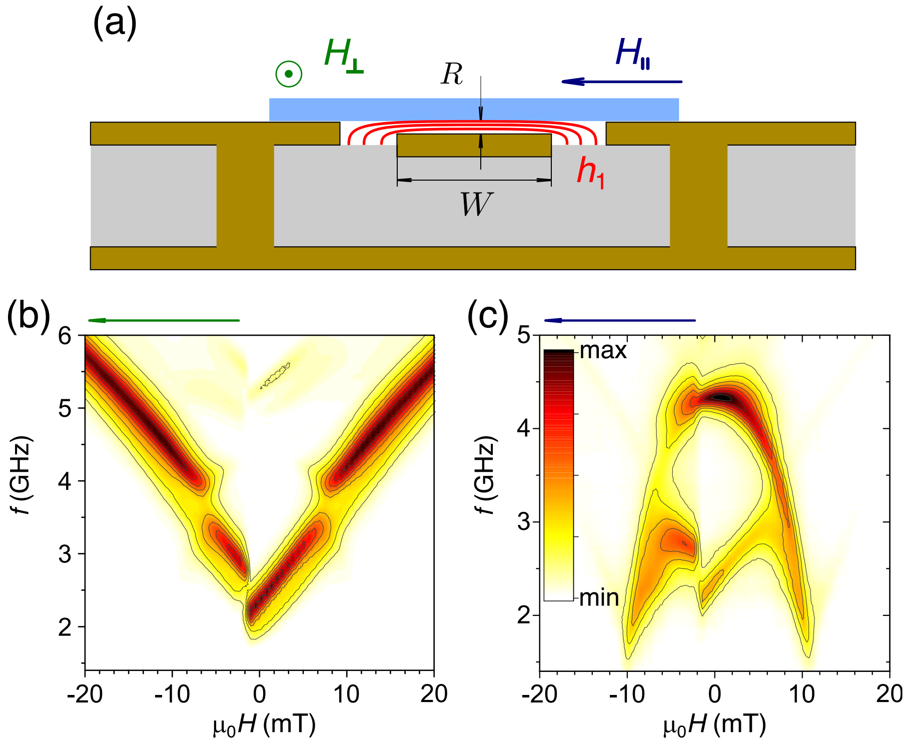


Fig. S6. Broadband ferromagnetic resonance measurements. (a) Measurement geometry. (b) Effective susceptibility measured in the (conventional) transverse pumping geometry. (c) Effective susceptibility measured in the longitudinal pumping geometry. The *(min,max)* values for color plots are $(0,-40)\times10^{-3}$, $(0,-15)\times10^{-3}$ for panels (b) and (c), respectively.

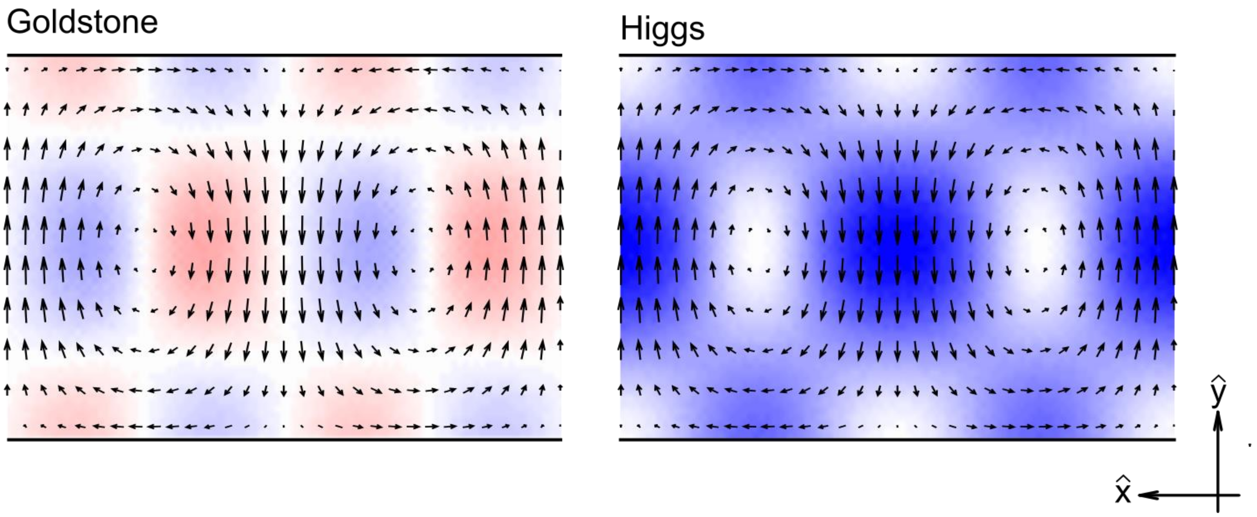


Fig. S7. Mumax3 simulation of the distribution of the longitudinal component of the dynamic magnetization of the Goldstone and Higgs modes. The value of $m_z = M_z - M_{eq,z}$ is shown in colors, from red (positive) to blue (negative). The black arrows depict the static transverse magnetization which defines the stripe domains. The profiles are obtained at $\mu_0 H$=7 mT by applying a sinusoidal excitation $h_y(x,t) = h_{y0}.\sin(2\pi\, f\, t - k_c\, x)$ with $f$=0.1 GHz (left panel) and $f$=3.5 GHz (right panel). Its amplitude is chosen to stay in the linear regime, being $\mu_0 h_{y0}$= 6 µT (left panel) and 0.1 µT (right panel).
